# Supplementary material for: Enhancing Data Quality through Self-learning on Imbalanced Financial Risk Data
Source: arXiv:2409.09792 source file (2024-09-15)
Supplement: Supplementary file 1 [file Appendix.tex]

% \newpage
% \newpage
% \section*{Appendix}
% \renewcommand\thesubsection{\Alph{subsection}}

%%In this section, we first 
% We now provide the table version in terms of the main results of TriEnhance for clear illustration.
% \textbf{Appendix}

\begin{table*}[!h]
    \centering
    \footnotesize 
    \caption{The table version in terms of the main results of TriEnhance}
    \begin{tabular}{llcccccc} 
    \toprule
    Dataset & Model & AUC & Accuracy & Recall & Precision & F1 & KS \\
    \midrule
    \multirow{8}{*}{BLSD} 
    & DT & 0.7372$\pm$0.0034 & 0.8121$\pm$0.0016 & 0.9742$\pm$0.0040 & 0.8180$\pm$0.0014 & 0.8893$\pm$0.0012 & 0.3162$\pm$0.0065 \\
    & TriEnhance\_DT & 0.7411$\pm$0.0023 & 0.8175$\pm$0.0010 & 0.9900$\pm$0.0044 & 0.8144$\pm$0.0021 & 0.8937$\pm$0.0008 & 0.3169$\pm$0.0097 \\
    & RF & 0.7621$\pm$0.0017 & 0.8205$\pm$0.0015 & 0.9987$\pm$0.0007 & 0.8125$\pm$0.0016 & 0.8961$\pm$0.0007 & 0.3537$\pm$0.0029 \\
    & TriEnhance\_RF & 0.7562$\pm$0.0004 & 0.8201$\pm$0.0015 & 0.9999$\pm$0.0001 & 0.8166$\pm$0.0013 & 0.8960$\pm$0.0008 & 0.3447$\pm$0.0024 \\
    & LGB & 0.7662$\pm$0.0011 & 0.8200$\pm$0.0013 & 0.9973$\pm$0.0012 & 0.8128$\pm$0.0015 & 0.8957$\pm$0.0006 & 0.3602$\pm$0.0044 \\
    & TriEnhance\_LGB & 0.7643$\pm$0.0009 & 0.8201$\pm$0.0015 & 0.9993$\pm$0.0005 & 0.8119$\pm$0.0014 & 0.8959$\pm$0.0007 & 0.3571$\pm$0.0036 \\
    & LR & 0.6969$\pm$0.0035 & 0.8161$\pm$0.0015 & 0.9941$\pm$0.0005 & 0.8111$\pm$0.0014 & 0.8934$\pm$0.0007 & 0.2647$\pm$0.0042 \\
    & TriEnhance\_LR & 0.6865$\pm$0.0056 & 0.8146$\pm$0.0030 & 0.9912$\pm$0.0029 & 0.8113$\pm$0.0013 & 0.8923$\pm$0.0018 & 0.2326$\pm$0.0096 \\
    \midrule
    \multirow{8}{*}{CCFD} 
    & DT & 0.8335$\pm$0.0250 & 0.9993$\pm$0.0001 & 0.7398$\pm$0.0246 & 0.8584$\pm$0.0156 & 0.7947$\pm$0.0205 & 0.7540$\pm$0.0156 \\
    & TriEnhance\_DT & 0.9030$\pm$0.0103 & 0.9991$\pm$0.0001 & 0.8049$\pm$0.0106 & 0.6969$\pm$0.0362 & 0.7468$\pm$0.0251 & 0.8164$\pm$0.0182 \\
    & RF & 0.9787$\pm$0.0066 & 0.9996$\pm$0.0000 & 0.7846$\pm$0.0093 & 0.9510$\pm$0.0213 & 0.8597$\pm$0.0112 & 0.8875$\pm$0.0178 \\
    & TriEnhance\_RF & 0.9662$\pm$0.0029 & 0.9994$\pm$0.0000 & 0.8150$\pm$0.0070 & 0.8303$\pm$0.0139 & 0.8226$\pm$0.0100 & 0.8818$\pm$0.0076 \\
    & LGB & 0.7720$\pm$0.0441 & 0.9967$\pm$0.0010 & 0.6463$\pm$0.0476 & 0.3083$\pm$0.0867 & 0.4135$\pm$0.0824 & 0.6763$\pm$0.0624 \\
    & TriEnhance\_LGB & 0.9607$\pm$0.0096 & 0.9993$\pm$0.0002 & 0.8110$\pm$0.0061 & 0.8024$\pm$0.0705 & 0.8055$\pm$0.0359 & 0.8726$\pm$0.0160 \\
    & LR & 0.9078$\pm$0.0146 & 0.9990$\pm$0.0001 & 0.6443$\pm$0.0511 & 0.7440$\pm$0.0511 & 0.6893$\pm$0.0285 & 0.7369$\pm$0.0188 \\
    & TriEnhance\_LR & 0.9355$\pm$0.0080 & 0.9923$\pm$0.0039 & 0.8211$\pm$0.0176 & 0.1838$\pm$0.0765 & 0.2947$\pm$0.1008 & 0.8277$\pm$0.0120 \\
    \midrule
    \multirow{8}{*}{GMSC} 
    & DT & 0.7717$\pm$0.0066 & 0.9310$\pm$0.0008 & 0.2009$\pm$0.0121 & 0.4630$\pm$0.0147 & 0.2802$\pm$0.0145 & 0.4778$\pm$0.0104 \\
    & TriEnhance\_DT & 0.7664$\pm$0.0039 & 0.9030$\pm$0.0085 & 0.3808$\pm$0.0291 & 0.3163$\pm$0.0258 & 0.3445$\pm$0.0147 & 0.4463$\pm$0.0108 \\
    & RF & 0.8629$\pm$0.0031 & 0.9363$\pm$0.0009 & 0.1729$\pm$0.0077 & 0.5795$\pm$0.0218 & 0.2663$\pm$0.0114 & 0.5711$\pm$0.0050 \\
    & TriEnhance\_RF & 0.8426$\pm$0.0027 & 0.9002$\pm$0.0031 & 0.4803$\pm$0.0177 & 0.3305$\pm$0.0064 & 0.3914$\pm$0.0016 & 0.5334$\pm$0.0019 \\
    & LGB & 0.8644$\pm$0.0028 & 0.9371$\pm$0.0006 & 0.1850$\pm$0.0076 & 0.5941$\pm$0.0131 & 0.2821$\pm$0.0099 & 0.5766$\pm$0.0044 \\
    & TriEnhance\_LGB & 0.8431$\pm$0.0028 & 0.9139$\pm$0.0035 & 0.4125$\pm$0.0159 & 0.3714$\pm$0.0138 & 0.3905$\pm$0.0026 & 0.5357$\pm$0.0069 \\
    & LR & 0.6855$\pm$0.0085 & 0.9332$\pm$0.0000 & 0.0199$\pm$0.0074 & 0.5023$\pm$0.0099 & 0.0382$\pm$0.0136 & 0.2680$\pm$0.0136 \\
    & TriEnhance\_LR & 0.7812$\pm$0.0094 & 0.9208$\pm$0.0099 & 0.3252$\pm$0.0573 & 0.4041$\pm$0.0701 & 0.3533$\pm$0.0159 & 0.4322$\pm$0.0120 \\
    \midrule
    \multirow{8}{*}{SFDFD} 
    & DT & 0.9767$\pm$0.0112 & 0.9997$\pm$0.0000 & 0.7626$\pm$0.0090 & 0.9680$\pm$0.0110 & 0.8530$\pm$0.0039 & 0.8813$\pm$0.0303 \\
    & TriEnhance\_DT & 0.9932$\pm$0.0008 & 0.9957$\pm$0.0005 & 0.9799$\pm$0.0017 & 0.2310$\pm$0.0195 & 0.3736$\pm$0.0255 & 0.9774$\pm$0.0015 \\
    & RF & 0.9980$\pm$0.0004 & 0.9996$\pm$0.0000 & 0.7309$\pm$0.0052 & 0.9939$\pm$0.0015 & 0.8423$\pm$0.0030 & 0.9630$\pm$0.0007 \\
    & TriEnhance\_RF & 0.9862$\pm$0.0002 & 0.9984$\pm$0.0008 & 0.7263$\pm$0.0396 & 0.4796$\pm$0.1511 & 0.5662$\pm$0.1164 & 0.8813$\pm$0.0088 \\
    & LGB & 0.5979$\pm$0.1635 & 0.9979$\pm$0.0010 & 0.4631$\pm$0.1867 & 0.3279$\pm$0.1650 & 0.3814$\pm$0.1988 & 0.5303$\pm$0.1830 \\
    & TriEnhance\_LGB & 0.9708$\pm$0.0036 & 0.9983$\pm$0.0004 & 0.6801$\pm$0.0148 & 0.4100$\pm$0.0691 & 0.5088$\pm$0.0515 & 0.8886$\pm$0.0067 \\
    & LR & 0.8801$\pm$0.0028 & 0.9983$\pm$0.0001 & 0.4298$\pm$0.0136 & 0.3594$\pm$0.0178 & 0.3914$\pm$0.0154 & 0.5440$\pm$0.0068 \\
    & TriEnhance\_LR & 0.9625$\pm$0.0057 & 0.9536$\pm$0.0024 & 0.8694$\pm$0.0180 & 0.0237$\pm$0.0016 & 0.0462$\pm$0.0031 & 0.8241$\pm$0.0208 \\
    \midrule
    \multirow{8}{*}{TCD} 
    & DT & 0.6893$\pm$0.0108 & 0.7995$\pm$0.0038 & 0.3822$\pm$0.0177 & 0.5706$\pm$0.0166 & 0.4574$\pm$0.0094 & 0.3468$\pm$0.0077 \\
    & TriEnhance\_DT & 0.7134$\pm$0.0227 & 0.8011$\pm$0.0223 & 0.3829$\pm$0.0546 & 0.5948$\pm$0.0897 & 0.4594$\pm$0.0073 & 0.3671$\pm$0.0241 \\
    & RF & 0.7764$\pm$0.0030 & 0.8189$\pm$0.0033 & 0.3585$\pm$0.0181 & 0.6691$\pm$0.0087 & 0.4667$\pm$0.0171 & 0.4291$\pm$0.0127 \\
    & TriEnhance\_RF & 0.7723$\pm$0.0030 & 0.8096$\pm$0.0092 & 0.4222$\pm$0.0422 & 0.6048$\pm$0.0523 & 0.4946$\pm$0.0149 & 0.4164$\pm$0.0075 \\
    & LGB & 0.7809$\pm$0.0025 & 0.8211$\pm$0.0025 & 0.3693$\pm$0.0173 & 0.6749$\pm$0.0090 & 0.4773$\pm$0.0146 & 0.4332$\pm$0.0118 \\
    & TriEnhance\_LGB & 0.7698$\pm$0.0020 & 0.8036$\pm$0.0024 & 0.4501$\pm$0.0126 & 0.5712$\pm$0.0059 & 0.5034$\pm$0.0098 & 0.4077$\pm$0.0073 \\
    & LR & 0.6539$\pm$0.0042 & 0.7789$\pm$0.0001 & 0.0011$\pm$0.0011 & 0.5000$\pm$0.5000 & 0.0021$\pm$0.0023 & 0.2273$\pm$0.0053 \\
    & TriEnhance\_LR & 0.6664$\pm$0.0069 & 0.7766$\pm$0.0053 & 0.0622$\pm$0.0344 & 0.5086$\pm$0.1011 & 0.1069$\pm$0.0538 & 0.2474$\pm$0.0063 \\
    \midrule
    \multirow{8}{*}{ZCD} 
    & DT & 0.7045$\pm$0.0409 & 0.8145$\pm$0.0099 & 0.4183$\pm$0.0444 & 0.4466$\pm$0.0259 & 0.4309$\pm$0.0279 & 0.4629$\pm$0.0402 \\
    & TriEnhance\_DT & 0.7177$\pm$0.0312 & 0.7992$\pm$0.0057 & 0.5882$\pm$0.0158 & 0.4295$\pm$0.0121 & 0.4965$\pm$0.0137 & 0.4880$\pm$0.0149 \\
    & RF & 0.8758$\pm$0.0037 & 0.8475$\pm$0.0014 & 0.3250$\pm$0.0107 & 0.5845$\pm$0.0085 & 0.4177$\pm$0.0090 & 0.6490$\pm$0.0041 \\
    & TriEnhance\_RF & 0.8667$\pm$0.0082 & 0.8187$\pm$0.0036 & 0.6880$\pm$0.0380 & 0.4734$\pm$0.0070 & 0.5606$\pm$0.0157 & 0.6462$\pm$0.0224 \\
    & LGB & 0.8760$\pm$0.0022 & 0.8448$\pm$0.0013 & 0.3571$\pm$0.0272 & 0.5611$\pm$0.0032 & 0.4361$\pm$0.0204 & 0.6451$\pm$0.0076 \\
    & TriEnhance\_LGB & 0.8674$\pm$0.0059 & 0.8332$\pm$0.0025 & 0.5348$\pm$0.0264 & 0.5042$\pm$0.0068 & 0.5188$\pm$0.0134 & 0.6309$\pm$0.0069 \\
    & LR & 0.8328$\pm$0.0069 & 0.8310$\pm$0.0013 & 0.0095$\pm$0.0104 & 0.5703$\pm$0.3925 & 0.0183$\pm$0.0199 & 0.6008$\pm$0.0031 \\
    & TriEnhance\_LR & 0.8237$\pm$0.0087 & 0.7344$\pm$0.0045 & 0.8746$\pm$0.0321 & 0.3757$\pm$0.0075 & 0.5256$\pm$0.0130 & 0.5953$\pm$0.0219 \\
    \bottomrule
    \end{tabular}
    \label{table: main_experiment_results}
    \vspace{-0.2cm}
\end{table*}
